# Supplementary material for: Robot Navigation in Unseen Spaces using an Abstract Map
Source: arXiv:2001.11684 source file (2020-05-15)
Supplement: Supplementary file 1 [file appendix.tex]

\appendix[Why Spring-Dynamics over Traditional Optimisation Techniques]

\todo{I have a page or so discussion that could go here showing the ``key toy map'' with a set initialisation, running it with each of the different optimisers, and showing how they all ``get stuck'', ending up with a much worse result than the spring dynamics. Personally I don't think it would be of value to the type of audience for this journal, but open to other opinions?}
